# Supplementary material for: SpinQuant: LLM quantization with learned rotations
Source: arXiv:2405.16406 source file (2025-02-20)
Supplement: Supplementary file 1 [file 12_gpu_latency.tex]

\begin{figure}[t!]
    \centering
    \includegraphics[width=0.9\linewidth]{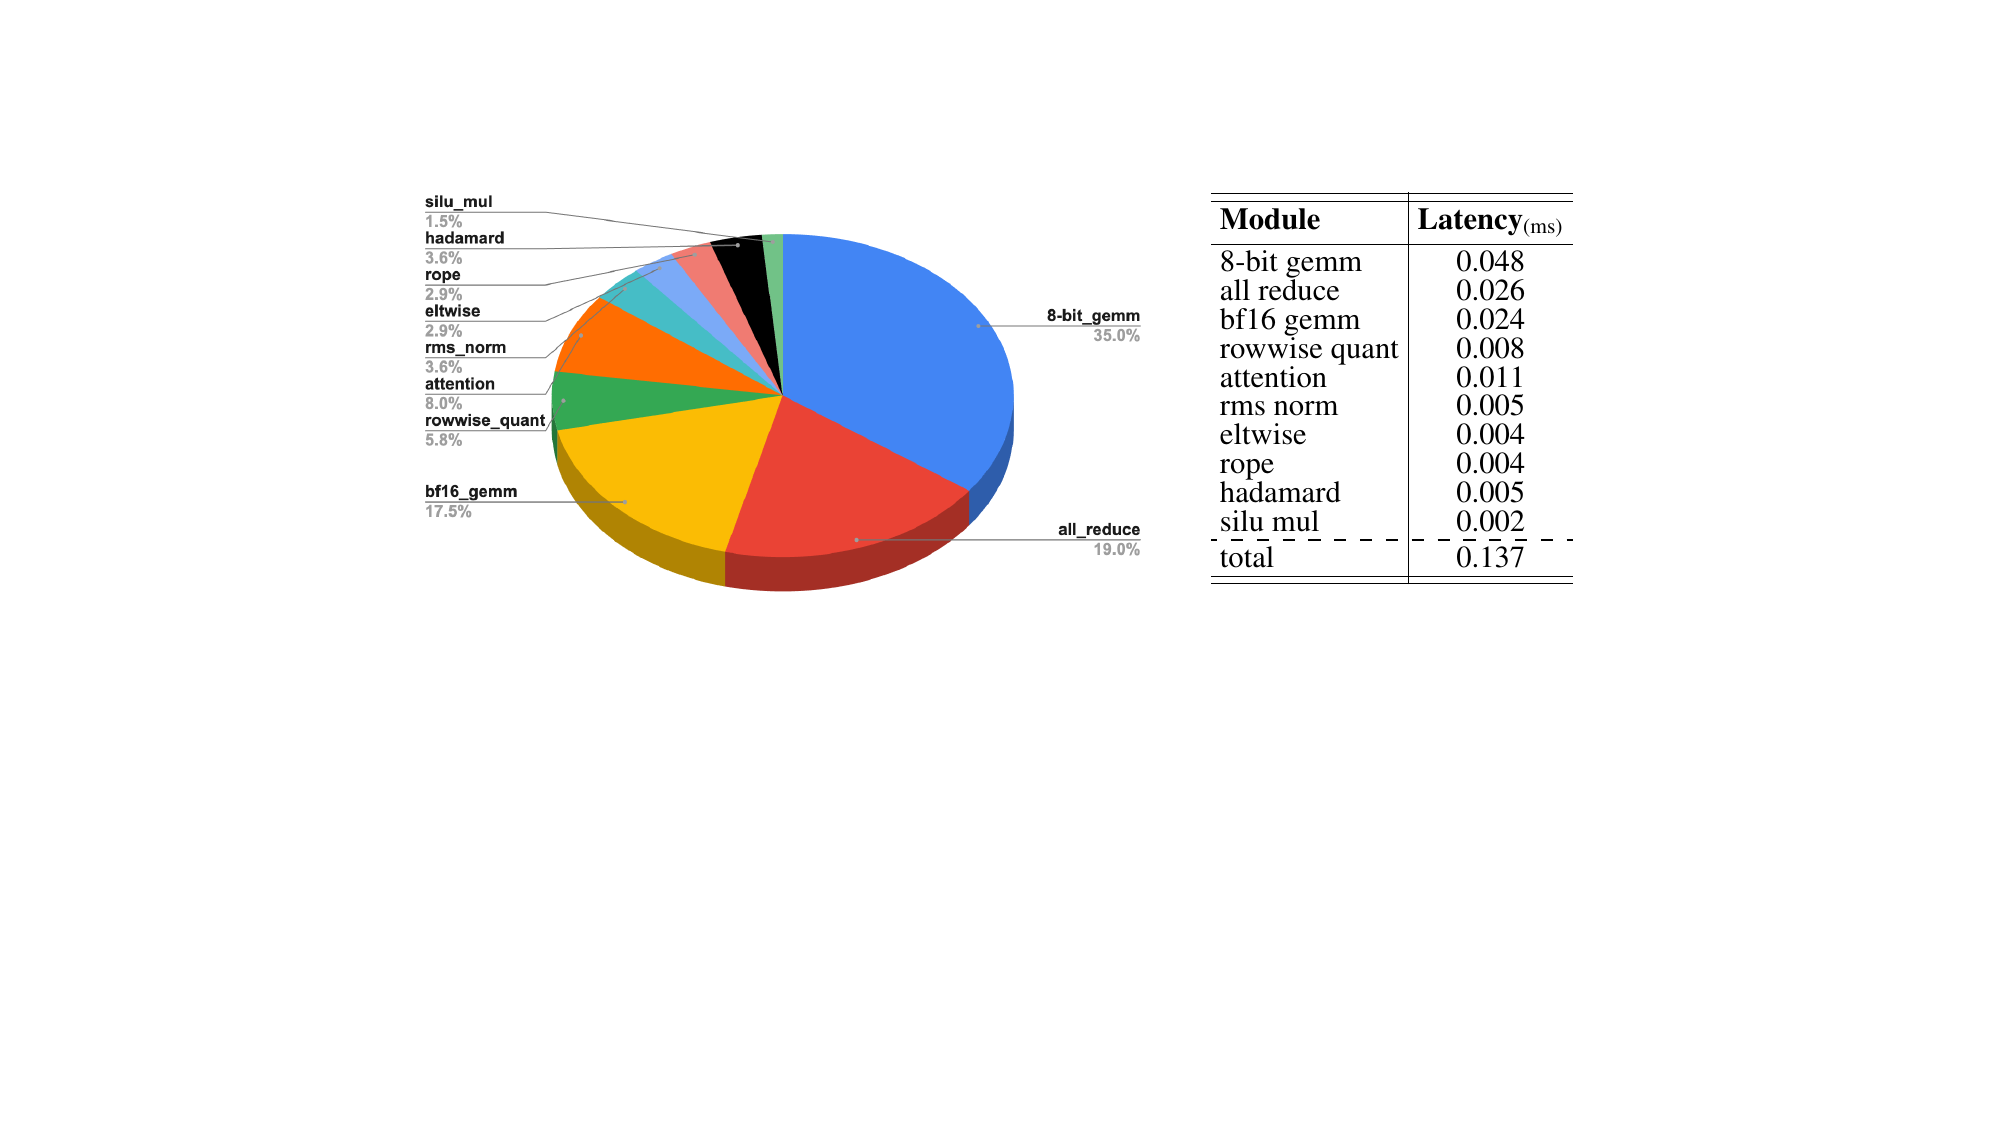}
    \caption{\small The latency measurement of LLaMA-3 70B model with 8 H100 GPUs }
    \label{fig:gpu_latency}
\end{figure}
